# Supplementary material for: Performance-based Trajectory Optimization for Path Following Control Using Bayesian Optimization
Source: arXiv:2103.15416 source file (2024-04-29)
Supplement: Supplementary file 1 [file appendix.tex]

\appendix
\section{Gaussian Process Regression}

Bayesian Optimization is a method to tune hyperparameter of function which are expensive to evaluate and that lack structure such as convexity or concavity. It make use of Gaussian Process to describe the unknown function and to find it's optimum in a minimum of iteration. The theoretical aspect introduced in this chapter is based on Rasmussen and Williams\cite{rasmussen2003gaussian} for the Gaussian Process modelling and on Frazier\cite{frazier2018tutorial} for the implementation of the Bayesian Optimization algorithm. \\

\subsection{Gaussian process}

According to \cite{rasmussen2003gaussian} the definition of a Gaussian Process \textit{is a collection of random variables, any finite number of which have (consistent) joint Gaussian distributions.}\\
As a gaussian distribution is a distribution over vectors,a Gaussian Porcess is a distribution over functions. It describe unknown function by a mean function and a covariance function, also called Kernel.

\begin{equation}
    \begin{bmatrix} f(x)\\  f(x') \end{bmatrix}\ \sim\
    \mathcal{N}
    \begin{pmatrix}
    \begin{bmatrix} \mu_0(x) \\  \mu_0(x') \end{bmatrix},
    &
    \begin{pmatrix}  \Sigma_0(x,x) & \Sigma_0(x,x') \\ \Sigma_0(x',x) & \Sigma_0(x',x')
    \end{pmatrix} 
    \end{pmatrix} 
\end{equation}

Gaussian process prior on a set of variables $x_1,...x_n$ and their evaluation $f(x_1),...f(x_n)$ : \\
\begin{equation}
    \begin{bmatrix} f(x_1)\\  \vdots \\ f(x_n) \end{bmatrix}\ \sim\
    \mathcal{N}
    \begin{pmatrix}
        \begin{bmatrix} \mu_0(x_1) \\ \vdots \\ \mu_0(x_n) \end{bmatrix},
        &\!\!\!\!\!\!\!\!\!\!\!\!\!\!\!
        \begin{bmatrix}  \Sigma_0(x_1,x_1) & \cdots & \Sigma_0(x_1,x_n) \\
        \vdots & \ddots & \vdots \\ \Sigma_0(x_n,x_1) & \cdots & \Sigma_0(x_n,x_n) \end{bmatrix} 
    \end{pmatrix} 
\end{equation}

posterior on $f(x')$ given $f(x_1),...f(x_n)$ stays normal and the mean $\mu_n(x')$ and  variance $\sigma_n^2$ and can be updated: \\
\begin{equation}
    f(x')|f(x_1,...x_n)\ \sim\ \mathcal{N} \begin{pmatrix} \mu_n(x'), & \sigma_n(x') \end{pmatrix}
\end{equation}
\begin{equation}
    \begin{split}
        &\mu_n(x')\ =\ \Sigma_0(x',x_{1:n})\Sigma_0(x_{1:n},x_{1:n})^{-1}(f(x_{1:n}) - \mu_0(x_{1:n}))\ +\ \mu_0(x')  \\ 
        &\sigma^{2}_n(x')\ =\ \Sigma_0(x',x')\ -\ \Sigma_0(x',x_{1:n})\Sigma_0(x_{1:n},x_{1:n})^{-1}\Sigma_0(x_{1:n},x')
    \end{split}
\end{equation}

\subsubsection{Choosing the mean kernel}

The covariance function $\Sigma_0$ is a function which decrease with the distance $\left \| x-x' \right \|$ namely if $\left \| x-x' \right \|< \left \| x -x'' \right \|$ then $\Sigma_0(x,x')> \Sigma_0(x,x'')$. There exist multiple possible choice for Kernel, for example Matern function or squared exponential. For this thesis, a squared exponential was chosen because it is versatile and can be used when we don't have many information about the function to optimize. It is defined as,

\begin{equation}
    \Sigma_0(x,x') = \alpha_0\text(exp)(-\left \| x-x' \right \|^2),
\end{equation}

where $\left \| x-x' \right \|^2 = \sum_{1}^{dim}\alpha_i(x_i-x_i')$ and $\alpha_{0:d}$ are the parameters of the kernel. They need to be evaluate and determine how quick the function is varying.

\subsubsection{Choosing the mean function}

The most commonly used mean function is a constant,

\begin{equation}
    \mu_0(x) = \mu .
\end{equation}

If there is information about the shape of the unknown function. It is possible to choose some linear or even polynomial kernel but this is not our case here. The constant mean function as one parameter which is simply $\mu$.

\subsubsection{Hyperparameter computation}

The hyperparameter of the mean and covariance function need to be determined. This can be done by maximizing the likelihood of the observation under the prior given the hyperparameters. This can be done at each iteration. 

\subsection{Acquisition function}

The acuqisition function is the key part of Bayesian optimization. Its role is to determine where the sample for the next function evaluation has to be taken. It has to trade off between exploitation and exploration of the function. One of the most popular acquisition function is the expected improvement. As it's name says it aims to find the candidate which maximize the expectation of improvement given the observation, the mean and the covariance function. Let $x^+$ be the current minimum of the function evaluation. The expected improvement is then,

\begin{equation}
    EI(x) = \mathop{\mathbb{E}}\left [ x^+ - min(x^+,F(x)) \right ].
\end{equation}

Where F(x) is the estimated value of x given the posterior Gaussian Process. An easy to compute way to evaluate the expected improvement which was developed by Mockus (1975)\cite{mockus} and popularized by Jones et al. (1998)\cite{article},

Finally the next candidate for the next function evaluation is the point which maximize this expected improvement function.

\subsection{Bayesian Optimization Algorithm}

\begin{algorithm}[h!]
        \DontPrintSemicolon
        \SetKwInput{kwInput}{Input}
        \SetKwInput{kwInit}{Initialization}
        \SetKwInput{kwMain}{Loop}
        \SetKwInput{kwOutput}{Output}
        \kwInput{
        \par
        \vspace{0.25cm}
            Initialization pairs of parameters and the associated value of the function to optimize
        }
        \kwInit{
        \par
        \vspace{0.25cm}
        \Indp{
            Prior estimation of the function, Gaussian description of the function to optimize, usually a Gaussian process
        }
        \vspace{0.25cm}
        }
        \kwMain{
        \par
        \vspace{0.25cm}
            \While {minimum criterion or maximum iteration is not reached}{
                - find the next quadidate to evaluate by maximizing the acquisition function of the prior\;
                - evaluate the function at the new quandidate\;
                - Update the posterior distribution of F\;
            }
        \vspace{0.25cm}
        }
        \kwOutput{
        \par
            Best quadidate which minimize the function.
        }
        \caption{Bayesian optimization principle}
\end{algorithm}

\subsection{Constrained Bayesian Optimization}
\label{sec:bo:const} 

For model predictive contouring control the performance of the controller is evaluate by the time it take to accomplish a trajectory and by the accuracy with which it can follow the trajectory. The time criterion is simple to describe as a cost for the bayesian optimization. But for the error along the trajectory, it would be nice to be able to find a way to include constraint and to find the minimum time which respect that constraint.\\
This can be done by updating the acquisition function to include the probability that the candidate will lead to a result respecting the constraint. 
A promising method was introduced by \cite{pmlr-v32-gardner14}. The principle is to include constraint to the bayesian optimization problem. The way to achieve this is to also describe the constraint inequality with gaussian process and to weight the expected improvement function with the result of this gaussian process:\\

\begin{itemize}
    \item non feasible point = 0
    \item low feasibility expectation = $<<1$ 
    \item high feasibility expectation = 1 
\end{itemize}

The constraint function is of the same nature as the main function to minimize, very costly to evaluate and to present any particular structure expected the fact that it is continuous and it might result from the same experiment. Then it is possible to model the constraint function with a Gaussian Process the same way it is done for the main function. The Gausian prior on the previous evaluation can then also be updated after each new evaluation.   

posterior on $c(x')$ given $c(x_1),...c(x_n)$ stays normal and the mean $\mu_n(x')$ and  variance $\sigma_n^2$ and can be updated: \\
\begin{equation}
    c(x')|c(x_1,...x_n)\ \sim\ \mathcal{N} \begin{pmatrix} \mu_{n,c}(x'), & \sigma_{n,c}(x') \end{pmatrix}
\end{equation}
\begin{equation}
    \begin{split}
        &\mu_{n,c}(x')\ =\ \Sigma_{0,c}(x',x_{1:n})\Sigma_{0,c}(x_{1:n},x_{1:n})^{-1}(c(x_{1:n}) - \mu_{0,c}(x_{1:n}))\ +\ \mu_{0,c}(x')  \\ 
        &\sigma^{2}_{n,c}(x')\ =\ \Sigma_{n,c}(x',x')\ -\ \Sigma_{0,c}(x',x_{1:n})\Sigma_{0,c}(x_{1:n},x_{1:n})^{-1}\Sigma_{0,c}(x_{1:n},x')
    \end{split}
\end{equation}

We then introduce a function representing the probability that the constraint function will stay under the constraint boundary.

\begin{equation}
    \tilde{\Delta }(x)\ =\ Pr[c(x')<\gamma ]\ =\ \int_{-\infty }^{\gamma} p(c(x)|x',c(x_{1:n}))dc(x)
\end{equation}

Then the constrained expected improvement of the next candidate is the expected improvement weighted by this function $\tilde{\Delta}(x)$.

\begin{equation}
    EI_C(x')\ =\ \tilde{\Delta}(x')EI(x') 
\end{equation}

Because of this modification the Expected Improvement will then tend to focus on the region where the function is realisable in regard of the constraints.

\section{Cost and Constraints Definition}
